# Supplementary material for: Split Packing: Algorithms for Packing Circles with Optimal Worst-Case Density
Source: arXiv:1705.00924 source file (2018-06-27)
Supplement: Supplementary file 1 [file appendix.tex]

%\section{Example hat-in-hat packings}
%
%\begin{table}[H]
%    \caption{Hat-in-hat packings for different values of $a_1$ and $a_2$.}
%    \label{tab:hats-in-hat}
%
%    \begin{tabular}{cp{7cm}}
%        \begin{tikzpicture}[scale=1.8,baseline={([yshift={-\ht\strutbox}]current bounding box.north)},outer sep=0pt,inner sep=0pt]
%            \hatsinhat{\defaulta}{\defaultb}{1}{0}
%        \end{tikzpicture}
%        & When $a_2 = a$, the second hat is simply rounded to a circle of area $a$. By definition, this is the incircle of the container, so it can be packed.\\
%
%        \begin{tikzpicture}[scale=1.8,baseline={([yshift={-\ht\strutbox}]current bounding box.north)},outer sep=0pt,inner sep=0pt]
%            \hatsinhat{\defaulta}{\defaultb}{0.9}{0}
%        \end{tikzpicture}
%        & As $a_2$ gets smaller, the second hat gets less rounded, but still enough so that it can be packed. The other hat is a non-rounded triangle, which fits beside the second one.\\
%
%        \begin{tikzpicture}[scale=1.8,baseline={([yshift={-\ht\strutbox}]current bounding box.north)},outer sep=0pt,inner sep=0pt]
%            \hatsinhat{\defaulta}{\defaultb}{0.7}{0}
%        \end{tikzpicture}
%        & \\
%
%        \begin{tikzpicture}[scale=1.8,baseline={([yshift={-\ht\strutbox}]current bounding box.north)},outer sep=0pt,inner sep=0pt]
%            \hatsinhat{\defaulta}{\defaultb}{0.5}{0}
%        \end{tikzpicture}
%        & \\
%
%        \begin{tikzpicture}[scale=1.8,baseline={([yshift={-\ht\strutbox}]current bounding box.north)},outer sep=0pt,inner sep=0pt]
%            \hatsinhat{\defaulta}{\defaultb}{0.43}{0}
%        \end{tikzpicture}
%        & When $a_1$ and $a_2$ have a ratio as specified by the container's associated split key, the two hats are both non-rounded triangles, but they can still be packed.\\
%
%        \begin{tikzpicture}[scale=1.8,baseline={([yshift={-\ht\strutbox}]current bounding box.north)},outer sep=0pt,inner sep=0pt]
%            \hatsinhat{\defaulta}{\defaultb}{0.3}{0}
%        \end{tikzpicture}
%        & When $a_2$ gets smaller than specified by the split key, it is now the first container which is getting more rounded.\\
%
%        \begin{tikzpicture}[scale=1.8,baseline={([yshift={-\ht\strutbox}]current bounding box.north)},outer sep=0pt,inner sep=0pt]
%            \hatsinhat{\defaulta}{\defaultb}{0.1}{0}
%        \end{tikzpicture}
%        & As $a_1$ approaches $a$, it is now the first hat whose shape gets closer to a perfect $a$-circle.\\
%
%        \begin{tikzpicture}[scale=1.8,baseline={([yshift={-\ht\strutbox}]current bounding box.north)},outer sep=0pt,inner sep=0pt]
%            \hatsinhat{\defaulta}{\defaultb}{0}{0}
%        \end{tikzpicture}
%        & By the same argument as before, this circle can be packed.\\
%    \end{tabular}
%\end{table}

%\begin{figure}[H]
%    \begin{tabular}{cc}
%        \subfig[0.015]{example-circles-in-equilateral-1} &
%        \subfig[0.015]{example-circles-in-equilateral-2} \\
%        \subfig[0.015]{example-circles-in-equilateral-3} &
%        \subfig[0.015]{example-circles-in-equilateral-4} \\
%        \subfig[0.015]{example-circles-in-equilateral-5} &
%        \subfig[0.015]{example-circles-in-equilateral-6} \\
%    \end{tabular}
%    \caption{Example packings of various circle instances into an equilateral triangle produced by Split Packing.}
%    \label{fig:example-circles-in-equilateral}
%\end{figure}
%
%\begin{figure}
%    \begin{tabular}{cc}
%        \subfig[0.015]{example-circles-in-rect-1} &
%        \subfig[0.015]{example-circles-in-rect-2} \\
%        \subfig[0.015]{example-circles-in-rect-3} &
%        \subfig[0.015]{example-circles-in-rect-4} \\
%        \subfig[0.015]{example-circles-in-rect-5} &
%        \subfig[0.015]{example-circles-in-rect-6} \\
%    \end{tabular}
%    \caption{Example packings of various circle instances in a rectangle with aspect ratio 1:1.57 produced by Split Packing.}
%    \label{fig:example-circles-in-rect}
%\end{figure}
